# Supplementary material for: Inexact and Stochastic Generalized Conditional Gradient with Augmented Lagrangian and Proximal Step
Source: arXiv:2005.05158 source file (2020-05-11)
Supplement: Supplementary file 1 [file sec-appendix_2.tex]

%----------------------------------
% These commands allow Gummi to
% edit each piece individually
% and still maintain previews.
%----------------------------------
\ifdefined\COMPLETE
\else
\documentclass[12pt]{article}
\input{package_header} %file containing all the used libraries
\begin{document}
\fi
%----------------------------------
% Remove at your own risk!
% There is also a footer that ends
% the document if the main wasn't
% loaded.
%----------------------------------

%-----------------------------------------------------

\section{Appendix}
\begin{lemma}\label{lem:gamest}
Consider a positive sequence $\seq{u_k}$ which satisfies\fekn
\nnewq{\label{eq:uass}
u_{k+1}\leq \para{1-c\gamma_k^s}u_k + d\gamma_k^t,
}
for some real numbers $s$ and $t$ satisfying $0<s<\min\brac{1,t}$. If, in addition, the sequence $\seq{\gamma_k}$ satisfies\fekn
\nnewq{\label{eq:gamass}
\frac{\gamma_k}{\gamma_{k+1}}\leq 1+o\para{\gamma_k^s},
}
then, for $k$ sufficiently large, it holds,
\newq{
u_k \leq \frac{d}{c} \gamma_k^{t-s}+o\para{\gamma_k^{t-s}}
}
\end{lemma}
\begin{proof}
For each $k\in\N$, we denote $\nu_k\eqdef \gamma_k^{s-t}u_k - \frac{d}{c}$ such that $u_k = \gamma_k^{t-s}\para{\nu_k+\frac{d}{c}}$. Then, by \eqref{eq:uass},
\newq{
\nu_{k+1} = \gamma_{k+1}^{s-t}u_{k+1}-\frac{d}{c} \leq \gamma_{k+1}^{s-t}\para{\para{1-c\gamma_k^s}u_{k} + d\gamma_k^t}-\frac{d}{c} = \gamma_k^{s-t}\para{\frac{\gamma_k}{\gamma_{k+1}}}^{t-s}\para{\para{1-c\gamma_k^s}u_k + d\gamma_k^t}-\frac{d}{c}.
}
By \eqref{eq:gamass}, we then have\fekn
\newq{
\nu_{k+1}\leq \gamma_k^{s-t}\para{1+o\para{\gamma_{k}^s}}^{t-s}\para{\para{1-c\gamma_k^s}u_k+d\gamma_k^t}-\frac{d}{c}.
}
Substituting for $u_k$ using the definition of $\nu_k$ we find\fekn
\newq{
\nu_{k+1}\leq \gamma_k^{s-t}\para{1+o\para{\gamma_k^s}}^{t-s}\para{\para{1-c\gamma_k^s}\para{\nu_k+\frac{d}{c}}\gamma_k^{t-s}+d\gamma_k^t}-\frac{d}{c}.
}
Now, we take a Taylor expansion for the term $\para{1+o\para{\gamma_k}^s}^{t-s}\approx \para{1+o\para{\gamma_k^s}}$ to get, for $k$ sufficiently large,
\newq{
\nu_{k+1}\leq \gamma_k^{s-t}\para{1+o\para{\gamma_k^s}}\para{\para{1-c\gamma_k^s}\para{\nu_k+\frac{d}{c}}\gamma_k^{t-s} + d\gamma_k^t} - \frac{d}{c}.
}
We distribute the $\gamma_k^{s-t}$ and then expand parentheses,
\newq{
\nu_{k+1}&\leq \para{1+o\para{\gamma_k^s}}\para{\para{1-c\gamma_k^s}\para{\nu_k+\frac{d}{c}} + d\gamma_k^s}-\frac{d}{c}\\
&=\para{1-c\gamma_k^s}\nu_k + \para{1-c\gamma_k^s}\frac{d}{c} + d\gamma_k^s + o\para{\gamma_k^s}\para{\para{1-c\gamma_k^s}\para{\nu_k+\frac{d}{c}} + d\gamma_k^s} - \frac{d}{c}\\
&=\para{1-c\gamma_k^s}\nu_k + \para{1-c\gamma_k^s}\frac{d}{c} + d\gamma_k^s + o\para{\gamma_k^s}\para{1-c\gamma_k^s}\nu_k+ o\para{\gamma_k^s}\para{1-c\gamma_k^s}\frac{d}{c} + o\para{\gamma_k^s}d\gamma_k^s - \frac{d}{c} \\
&=\para{1-c\gamma_k^s+ o\para{\gamma_k^s}}\nu_k +o\para{\gamma_k^s}.
}
Fix $0<\tilde c<c$. Then, by definition of $o\para{\gamma_k^s}$, $\exists k_0\in\N$ such that, $\forall k>k_0$, $o\para{\gamma_k^s}\leq (c-\tilde{c})\gamma_k^s$. Then,
\newq{
\para{1-c\gamma_k^s+ o\para{\gamma_k^s}}\nu_k \leq \para{1-\tilde c \gamma_k^s}\nu_k.
}
From this we conclude, by \cite[Ch.2, Lemma~3]{polyak1987introduction}, that $\limsup\limits_k \nu_k \leq 0$.
Thus, by definition of $\nu_{k}$,
\newq{
u_{k+1}\leq \frac{d}{c}\gamma_k^{t-s}+o\para{\gamma_k^{t-s}}.
}
\end{proof}
%-----------------------------------------------------

%-----------------------
% Footer to allow Gummi
% to maintain previews
% for individual pieces
%-----------------------
\ifdefined\COMPLETE
\else
\end{document}
\fi
